# Supplementary material for: Enhancing the efficiency of polariton OLEDs in and beyond the single-excitation subspace
Source: arXiv:2404.04257 ancillary file (2024-10-17)
Supplement: Supplementary file 1 [file Supplementary_Information.pdf]

# Supplementary Information:
# Enhancing the efficiency of polariton OLEDs in and beyond the single-excitation subspace

*Siltanen et al.*

**Supplementary Note 1: Comments on the total RISC rate.**

The total RISC rate in the strong-coupling case, when considering the entire single-excitation subspace, can be written as $k_{RISC}^{tot.} = \frac{1}{N}\left[\left|\alpha^{(1)}\right|^2 k(\lambda_+, E_+ - E_t) + \left|\beta^{(1)}\right|^2 k(\lambda_-, E_- - E_t) + (N-1)k(\lambda_s, E_s - E_t)\right]$ or alternatively as $k_{RISC}^{tot.} = k_{RISC}^{s} + \Delta k_{RISC}$, where $\Delta k_{RISC} = k_{RISC}^{+} + k_{RISC}^{-} - k_{RISC}^{s}/N$ . If $k_{RISC}^{-} = k_{RISC}^{s}$, the energy gap $E_+ - E_t$ is so large that $k_{RISC}^{+} \approx 0$. Furthermore, if $N \gg 0$, we can absorb $k_{RISC}^{s}/N$ to $k_{RISC}^{s}$ and estimate that $k_{RISC}^{tot.} \approx 2k_{RISC}^{s}$. That is, if the LP gets populated at the same rate as the bare-film singlets, the triplets get *depopulated* twice as fast. Still, since we are interested in the bright states, we use the criterion $k_{RISC}^{-} = k_{RISC}^{s}$ for enhanced RISC. Similar argument holds for TTA.

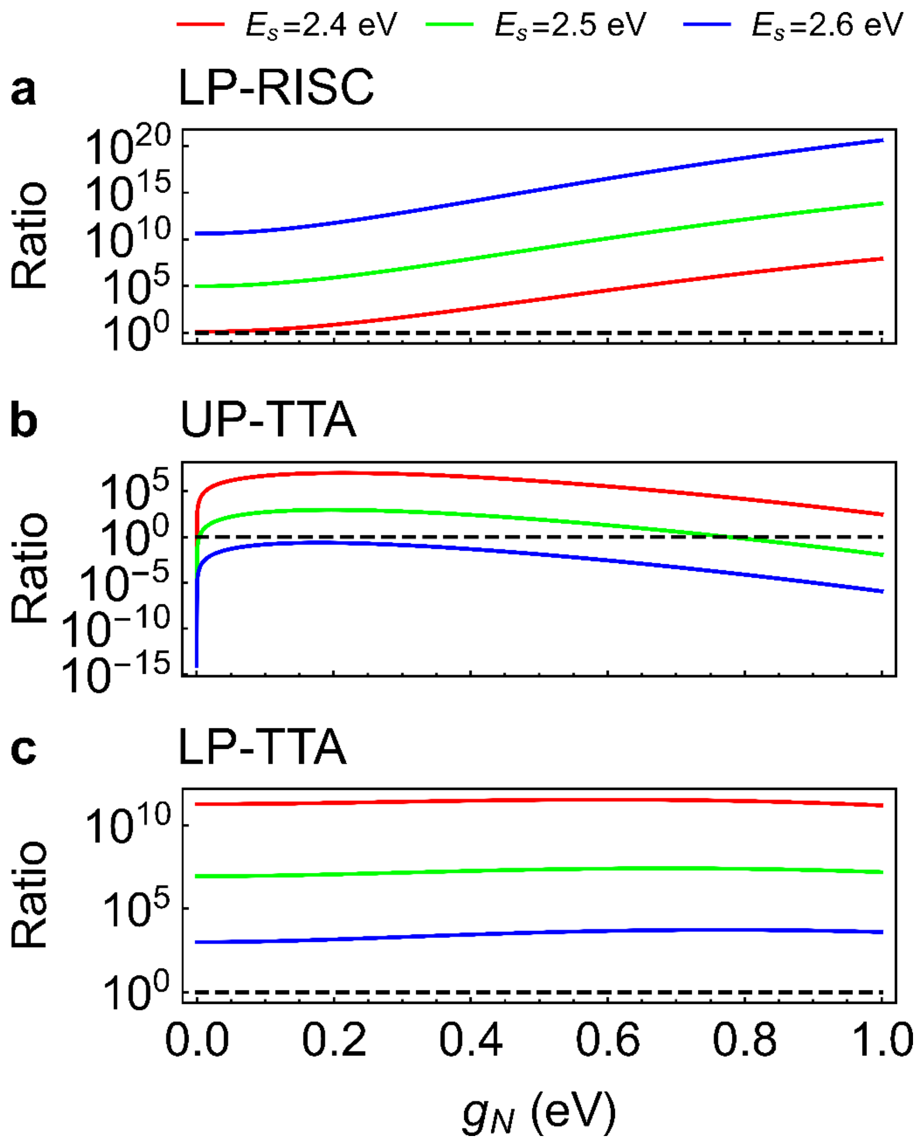


**Supplementary Figure 1: Polariton-to-singlet ratios of RISC and TTA rates. a,** $k_{RISC}^{-}/k_{RISC}^{s}$. **b,** $k_{TTA}^{+}/k_{TTA}^{s}$. **c,** $k_{TTA}^{-}/k_{TTA}^{s}$. The rates are enhanced above the black dashed line. The parameters are $N = 10^{10}$, $n_{\text{eff}} = 2$, $m = 1$, $L_c = 100$ nm, $k_{\|} = 0$, $T = 293$ K, $E_t = 1.80$ eV, $\lambda_s = 0.10$ eV, and $\lambda_{\pm} = 0.79$ eV.

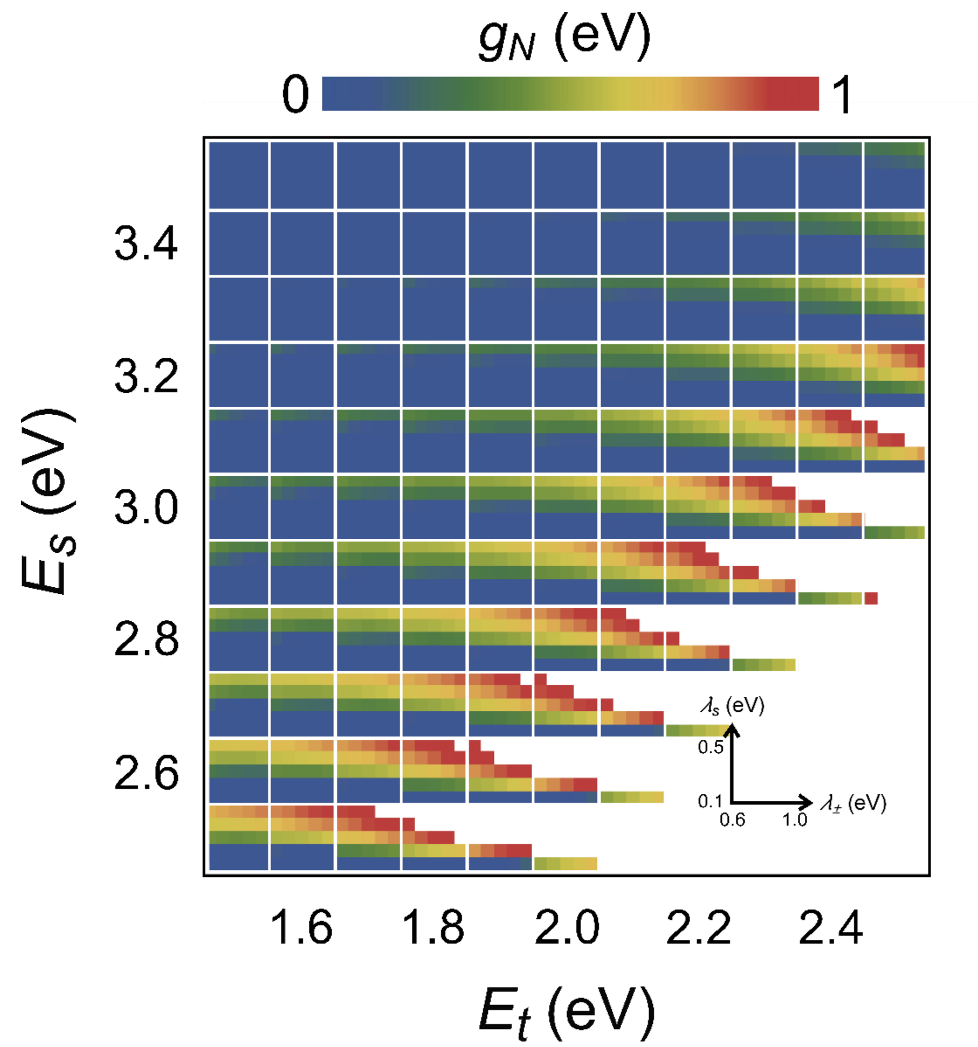


**Supplementary Figure 2: Detailed scan of LP-RISC.** The minimum values of $g_N$ required to achieve the same T-to-LP RISC rate as T-to-S with different singlet, triplet, and reorganization energies. The map is divided into 11×11 supercells that consist of 5×5 cells. For each supercell, the values of $\lambda_s$ and $\lambda_\pm$ are varied, while $E_s$ and $E_t$ are fixed. The parameters are $N = 10^{10}$, $n_{\text{eff}} = 2$, $m = 1$, $L_c = 100$ nm, $k_{\parallel} = 0$, and $T = 293$ K.

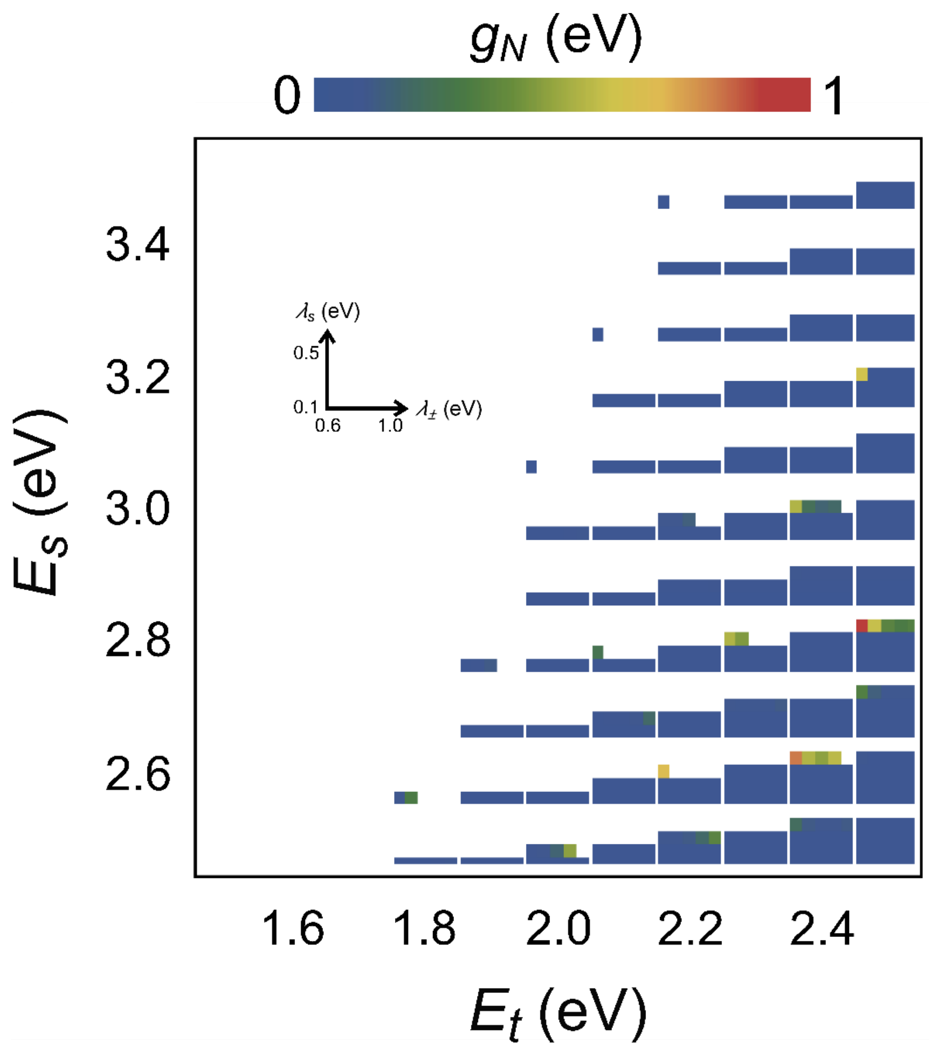


**Supplementary Figure 3: Detailed scan of UP-TTA.** The minimum values of $g_N$ required to achieve the same **S**-to-UP TTA rate as **S**-to-S with different singlet, triplet, and reorganization energies. The map is divided into 11×11 supercells that consist of 5×5 cells. For each supercell, the values of $\lambda_s$ and $\lambda_\pm$ are varied, while $E_s$ and $E_t$ are fixed. The parameters are $N = 10^{10}$, $n_{\text{eff}} = 2$, $m = 1$, $L_c = 100$ nm, $k_{\parallel} = 0$, and $T = 293$ K.

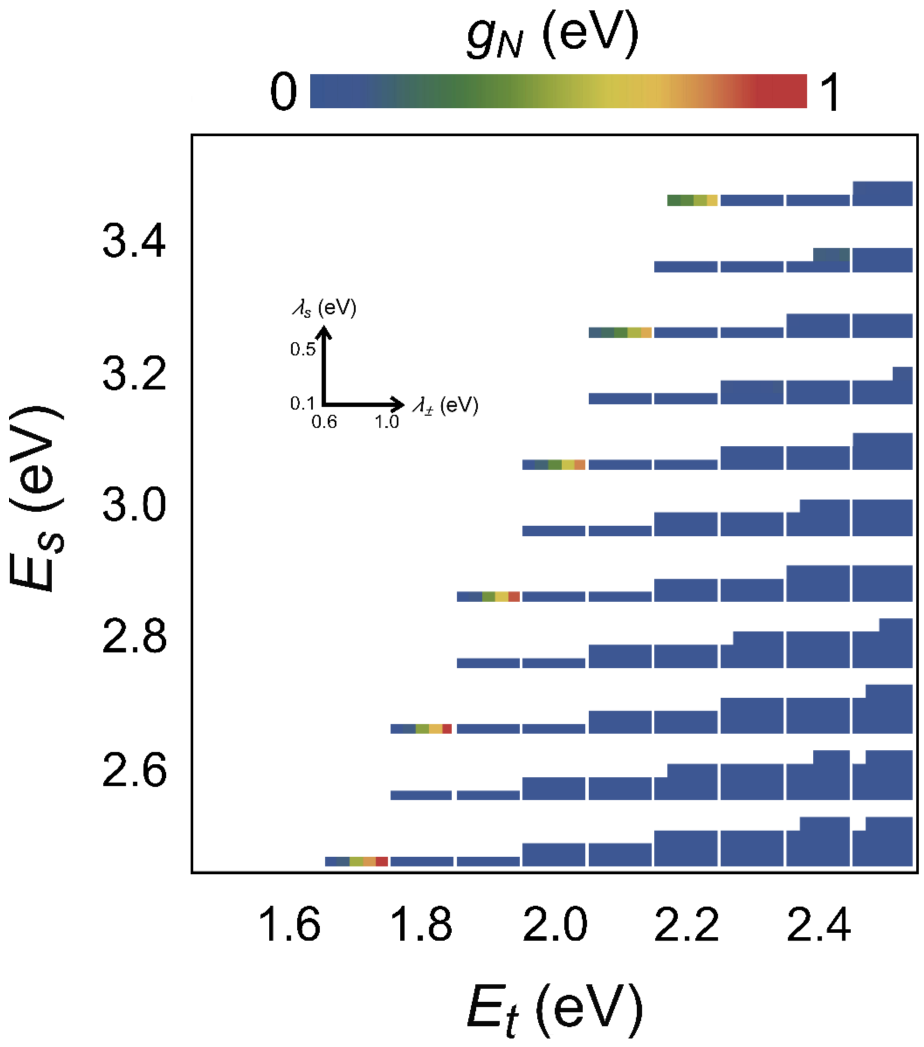


**Supplementary Figure 4: Detailed scan of LP-TTA.** The minimum values of $g_N$ required to achieve the same **S**-to-LP TTA rate as **S**-to-S with different singlet, triplet, and reorganization energies. The map is divided into 11×11 supercells that consist of 5×5 cells. For each supercell, the values of $\lambda_s$ and $\lambda_\pm$ are varied, while $E_s$ and $E_t$ are fixed. The parameters are $N = 10^{10}$, $n_{\text{eff}} = 2$, $m = 1$, $L_c = 100$ nm, $k_{\|} = 0$, and $T = 293$ K.

**Supplementary Table 1: Experimental parameters.** When calculating the Marcus rates in the main text, we used $E_S^0$ (0-0 transition) for the bare-film cases and $E_S^{abs}$ (absorption) for the cavity case, since we assumed decoupling from the vibrational degrees of freedom. *The cavity-mode energy $E_c$ of tetracene is actually the energy of a surface lattice resonance, but the same analysis holds.

| **Molecule** | $\boldsymbol{T}$ **(K)** | $\boldsymbol{E_S^{abs}}$ **(eV)** | $\boldsymbol{E_S^0}$ **(eV)** | $\boldsymbol{E_t^0}$ **(eV)** | $\boldsymbol{E_c}$ **(eV)** | $\boldsymbol{g_N}$ **(eV)** |
|---|---|---|---|---|---|---|
| Erythrosine B | 312 | 2.32 | 2.25 | 1.93 | 2.42 | 0.19 |
| DABNA-2 | 181 | 2.79 | 2.72 | 2.60 | 2.45 | 0.22 |
| Tetracene | 293 | 2.38 | 2.37 | 1.28 | 2.35* | 0.11 |
| $DPP(PhCl)_2$ | 298 | 2.49 | 2.26 | 1.10 | 2.21 | 0.22 |
| 3DPA3CN | 293 | 2.92 | 2.51 | 2.41 | 2.56 | 0.23 |
| TDAF | 293 | 3.54 | 3.22 | 2.38 | 2.93 | 0.48 |
